# Supplementary material for: Instance-Adaptive and Geometric-Aware Keypoint Learning for Category-Level 6D Object Pose Estimation
Source: arXiv:2403.19527 source file (2024-03-28)
Supplement: Supplementary file 1 [file suppl.tex]

\clearpage
\setcounter{page}{1}
\maketitlesupplementary
% 0. More implementation details
% 1. FPS/Memory Study
% 2. Per Category Results Table + Curve
% 3. More visualization on REAL275 dataset. 
% 4. Keypoint Heatmap Visualization
\section{More implementation details}
% pn++ CNN total iteration B1:B2 
Here we offer more implementation details about our AG-Pose. 
For the Feature Extractor, we use a PSP Network \cite{zhao2017psp} based on ResNet-18 \cite{he2016resnet} to extract the image feature and implement the PointNet++ \cite{qi2017pointnet++} with 4 set abstract layers and multi-scale grouping to extract the point feature. 
For the IAKD, the attention layers contains of four attention blocks, and each of them is a standard attention operation \cite{vaswani2017attention} with $d_{model} = 256$ and $num\_heads = 4$. 
For other training details, we train our network for 50 epochs with a total of 200,000 iterations. The batch size is set as 24, with a ratio of 3:1 between real and synthetic data. 
All experiments are conducted on a single RTX 3090 GPU with an Intel Xeon Gold 6248R @ 4.000 GHz CPU. We implement our code using PyTorch 1.12.1 and CUDA 11.3. 
\section{Symmetry handling}
The issue of object symmetry is common in pose estimation. To handle it, following \cite{Tian2020spd}, we map ambiguous rotations to a canonical one. Since all symmetric objects in NOCS datasets \cite{Wang2019nocs} exhibit continuous symmetry along the y-axis, for a rotation $R$, the above process is as follows,
\begin{gather}
    \textit{Map}(R) = R{\hat{S}}, \\
    {\hat{S}} = 
    \begin{bmatrix}
        cos\hat{\theta} \, &0 \, &-sin\hat{\theta} \\ 
        0 \, &1 \, &0 \\ 
        sin\hat{\theta} \, &0 \, &cos\hat{\theta} \\ 
    \end{bmatrix},
    \\
    \hat{\theta} = arctan 2(R_{13}-R_{31}, R_{11}+R_{33}).
\end{gather}

\section{Accuracy, memory usage, total parameters and inference speed of models with different $N_{kpt}$}
To demonstrate the efficiency and scalability of our AG-Pose, we show the quantitative results of the accuracy, GPU memory usage during training, total parameters and inference speed of our model with different number of keypoints $N_{kpt}$ in Table \ref{tab:ab_supp}. 
As demonstrated by the results, the accuracy of our AG-Pose improves when increasing $N_{kpt}$.
It is worth noting that the increment of the GPU memory usage, the total parameters and the computational overhead of our model are slight and acceptable. 
Specifically, when we lift the number of keypoints $N_{kpt}$ from 16 to 128, the total parameters of the model just increase by less than $1\%$,
and the increase in GPU memory usage is also affordable. 
Additional, the inference speed of our model only decreases by less than $10\%$. 
We attribute this to that: 1) The number of keypoints $N_{kpt}$ is quite small compared to the size of point cloud $N$. Using this sparse set of keypoints to represent the shapes of objects is effective and efficient. 2) The two-stage feature aggregation pipeline in proposed GAFA module is efficient, which can inject local and global geometric information into keypoints with a low computational burden. 

\section{Per-category results}
The NOCS datasets \cite{Wang2019nocs} contains six different categories: bottle, bowl, camera, can, laptop and mug. 
We show the per-category and the average results of our AG-Pose on the REAL275 and
CAMERA25 datasets in Table \ref{tab:REAL275_per_cat} and Table \ref{tab:CAMERA25_per_cat}, respectively. 
It is worth noting that we train a single model for all categories as \cite{lin2022dpdn,query6dof,Zheng2023hspose}.  
\section{Keypoint heatmaps visualization}
Here we visualize the query-instance heatmap $\mathbf{H}$ in the proposed Instance-Adaptive Keypoint Detector in Figure \ref{fig:heatmap}. 
We use the bottle category as an example. 
Specifically, we draw the heatmaps for the same query across different instances as well as heatmaps for different queries on the same instance. 
As shown in the Figure, different queries can focus on different parts of the input instance to comprehensively depict the shape of the object. 
On the other hand, the same query tends to focus on regions with similar structures across different instances, which demonstrates the generalizability of our IAKD within the specific category. 

\section{More visualization on REAL275}
Here we visualize more pose predictions of our AG-Pose in Figure \ref{fig:more_viz}. 
In particular, we choose four images per scene for all six unseen scenes in the REAL275 validation set, in which red/green indicates the predicted/gt results.

\begin{table}[h]
    \setlength{\tabcolsep}{4pt}
    \caption{\textbf{
        Comparisons between models with different $N_{kpt}$.}
        }
    \label{tab:ab_supp}
    \centering
    \begin{tabular}{c|cc|c|c|c}
        \hline
        $N_{kpt}$ & $IoU_{75}$         & $5^{\circ} \, 2 \, \textbf{cm}$             & Memory & Parameters & Speed(FPS) \\ \hline
        16     & 78            & 47.9          & 11.6G      & 207,529,575        & 30.61      \\
        32     & 78.3          & 48.8          & 12.1G      & 207,541,863        & 30.33      \\
        64     & \textbf{79.7} & 51            & 13.4G      & 207,566,439        & 29.88      \\
        96     & 79.5          & \textbf{54.7} & 14.4G      & 207,591,015        & 27.98      \\
        128    & 78.8          & 52.8          & 16.4G      & 207,615,591        & 27.58      \\ \hline
        \end{tabular}
\end{table} 
\begin{table}[h]
    \setlength{\tabcolsep}{3pt}
    \caption{\textbf{
        Per-category results of AG-Pose on REAL275.}
        }
    \label{tab:REAL275_per_cat}
    \centering
    \begin{tabular}{c|cc|cccc}
        \hline
        category & $IoU_{50}$ & $IoU_{75}$ & $5^{\circ} \, 2 \, \textbf{cm}$  & $5^{\circ} \, 5 \, \textbf{cm}$  & $10^{\circ} \, 2 \, \textbf{cm}$ & $10^{\circ} \, 5 \, \textbf{cm}$ \\ \hline
        bottle   & 57.7  & 50.3  & 62   & 64.9 & 83.4 & 88   \\
        bowl     & 100   & 100   & 88.7 & 94.3 & 94.1 & 99.7 \\
        camera   & 90.8  & 82.9  & 1.2  & 1.3  & 24.8 & 27.3 \\
        can      & 71.3  & 71.2  & 83.4 & 85.3 & 96.3 & 98.6 \\
        laptop   & 83.3  & 74.1  & 59.6 & 91.1 & 61.2 & 95.6 \\
        mug      & 99.4  & 98.5  & 32.9 & 33.4 & 88.3 & 89.3 \\ \hline
        average  & 83.7  & 79.5  & 54.7 & 61.7 & 74.7 & 83.1 \\ \hline
        \end{tabular}
    \end{table} 
\begin{table}[h]
    \setlength{\tabcolsep}{3pt}
\caption{\textbf{
    Per-category results of AG-propose on CAMERA25.}
    }
\label{tab:CAMERA25_per_cat}
\centering
\begin{tabular}{c|cc|cccc}
    \hline
    category & $IoU_{50}$ & $IoU_{75}$ & $5^{\circ} \, 2 \, \textbf{cm}$  & $5^{\circ} \, 5 \, \textbf{cm}$  & $10^{\circ} \, 2 \, \textbf{cm}$ & $10^{\circ} \, 5 \, \textbf{cm}$ \\ \hline
    bottle   & 93.7  & 91.4  & 80.9 & 96.4 & 82.3 & 99   \\
    bowl     & 96.9  & 96.7  & 98.7 & 99   & 99.7 & 99.8 \\
    camera   & 89.2  & 84.3  & 57   & 60.9 & 73.6 & 81.1 \\
    can      & 92.1  & 92    & 99.7 & 99.8 & 99.7 & 99.9 \\
    laptop   & 97.5  & 90.8  & 76.1 & 85.9 & 80.6 & 92.4 \\
    mug      & 93.6  & 92.7  & 54.5 & 54.6 & 77.1 & 77.3 \\ \hline
    average  & 93.8  & 91.3  & 77.8 & 82.8 & 85.5 & 91.6 \\ \hline
    \end{tabular}
\end{table}

\begin{figure*}[t]
    \begin{center}
    \includegraphics[width=0.8\textwidth]{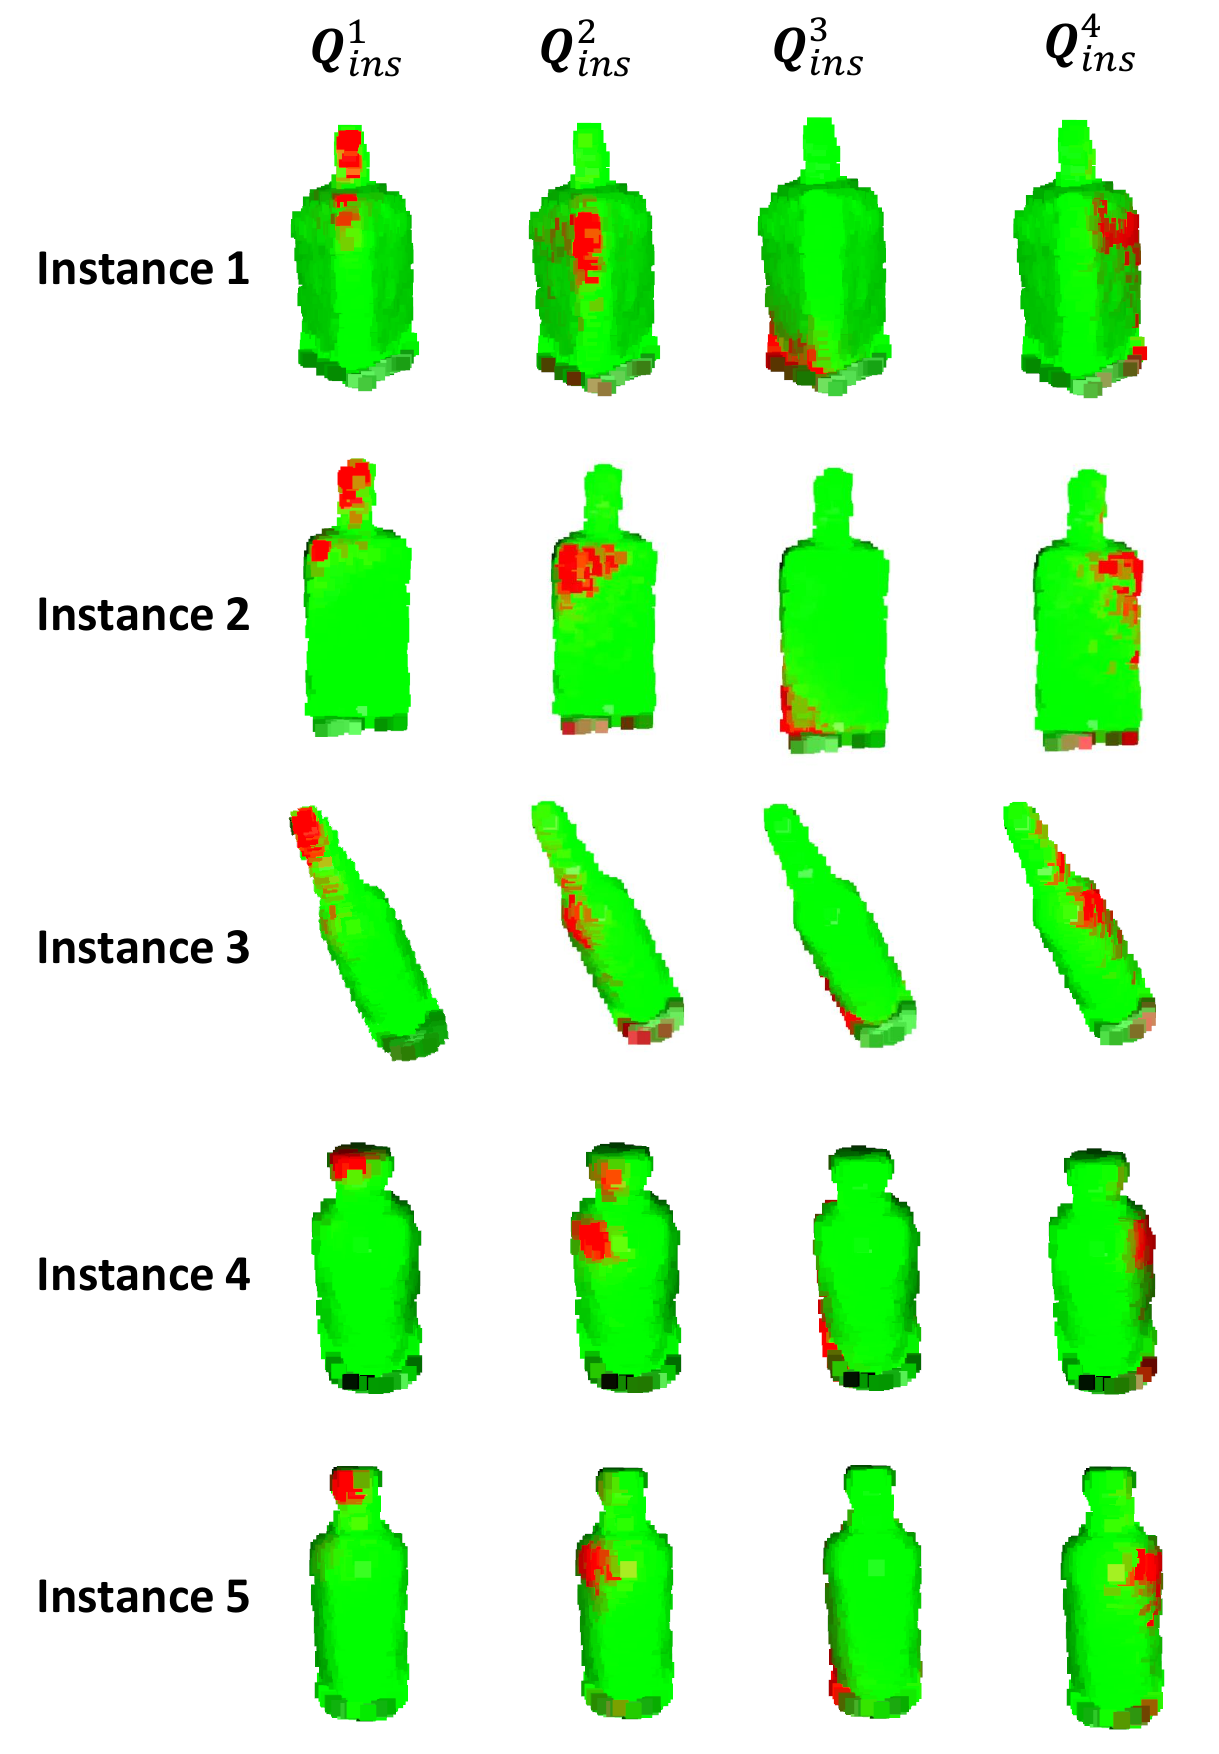}
    \caption{\textbf{Query-instance heatmaps in the proposed IAKD.} Each row represents the heatmaps for different queries on a same instance. Each column represents the heatmaps for a same query across different input instances. Red/green indicates a large/small weight.}
    \label{fig:heatmap} 
    \end{center}
    \vspace{-0.25in}
\end{figure*}

\begin{figure*}[t]
    \begin{center}
    \includegraphics[width=\textwidth]{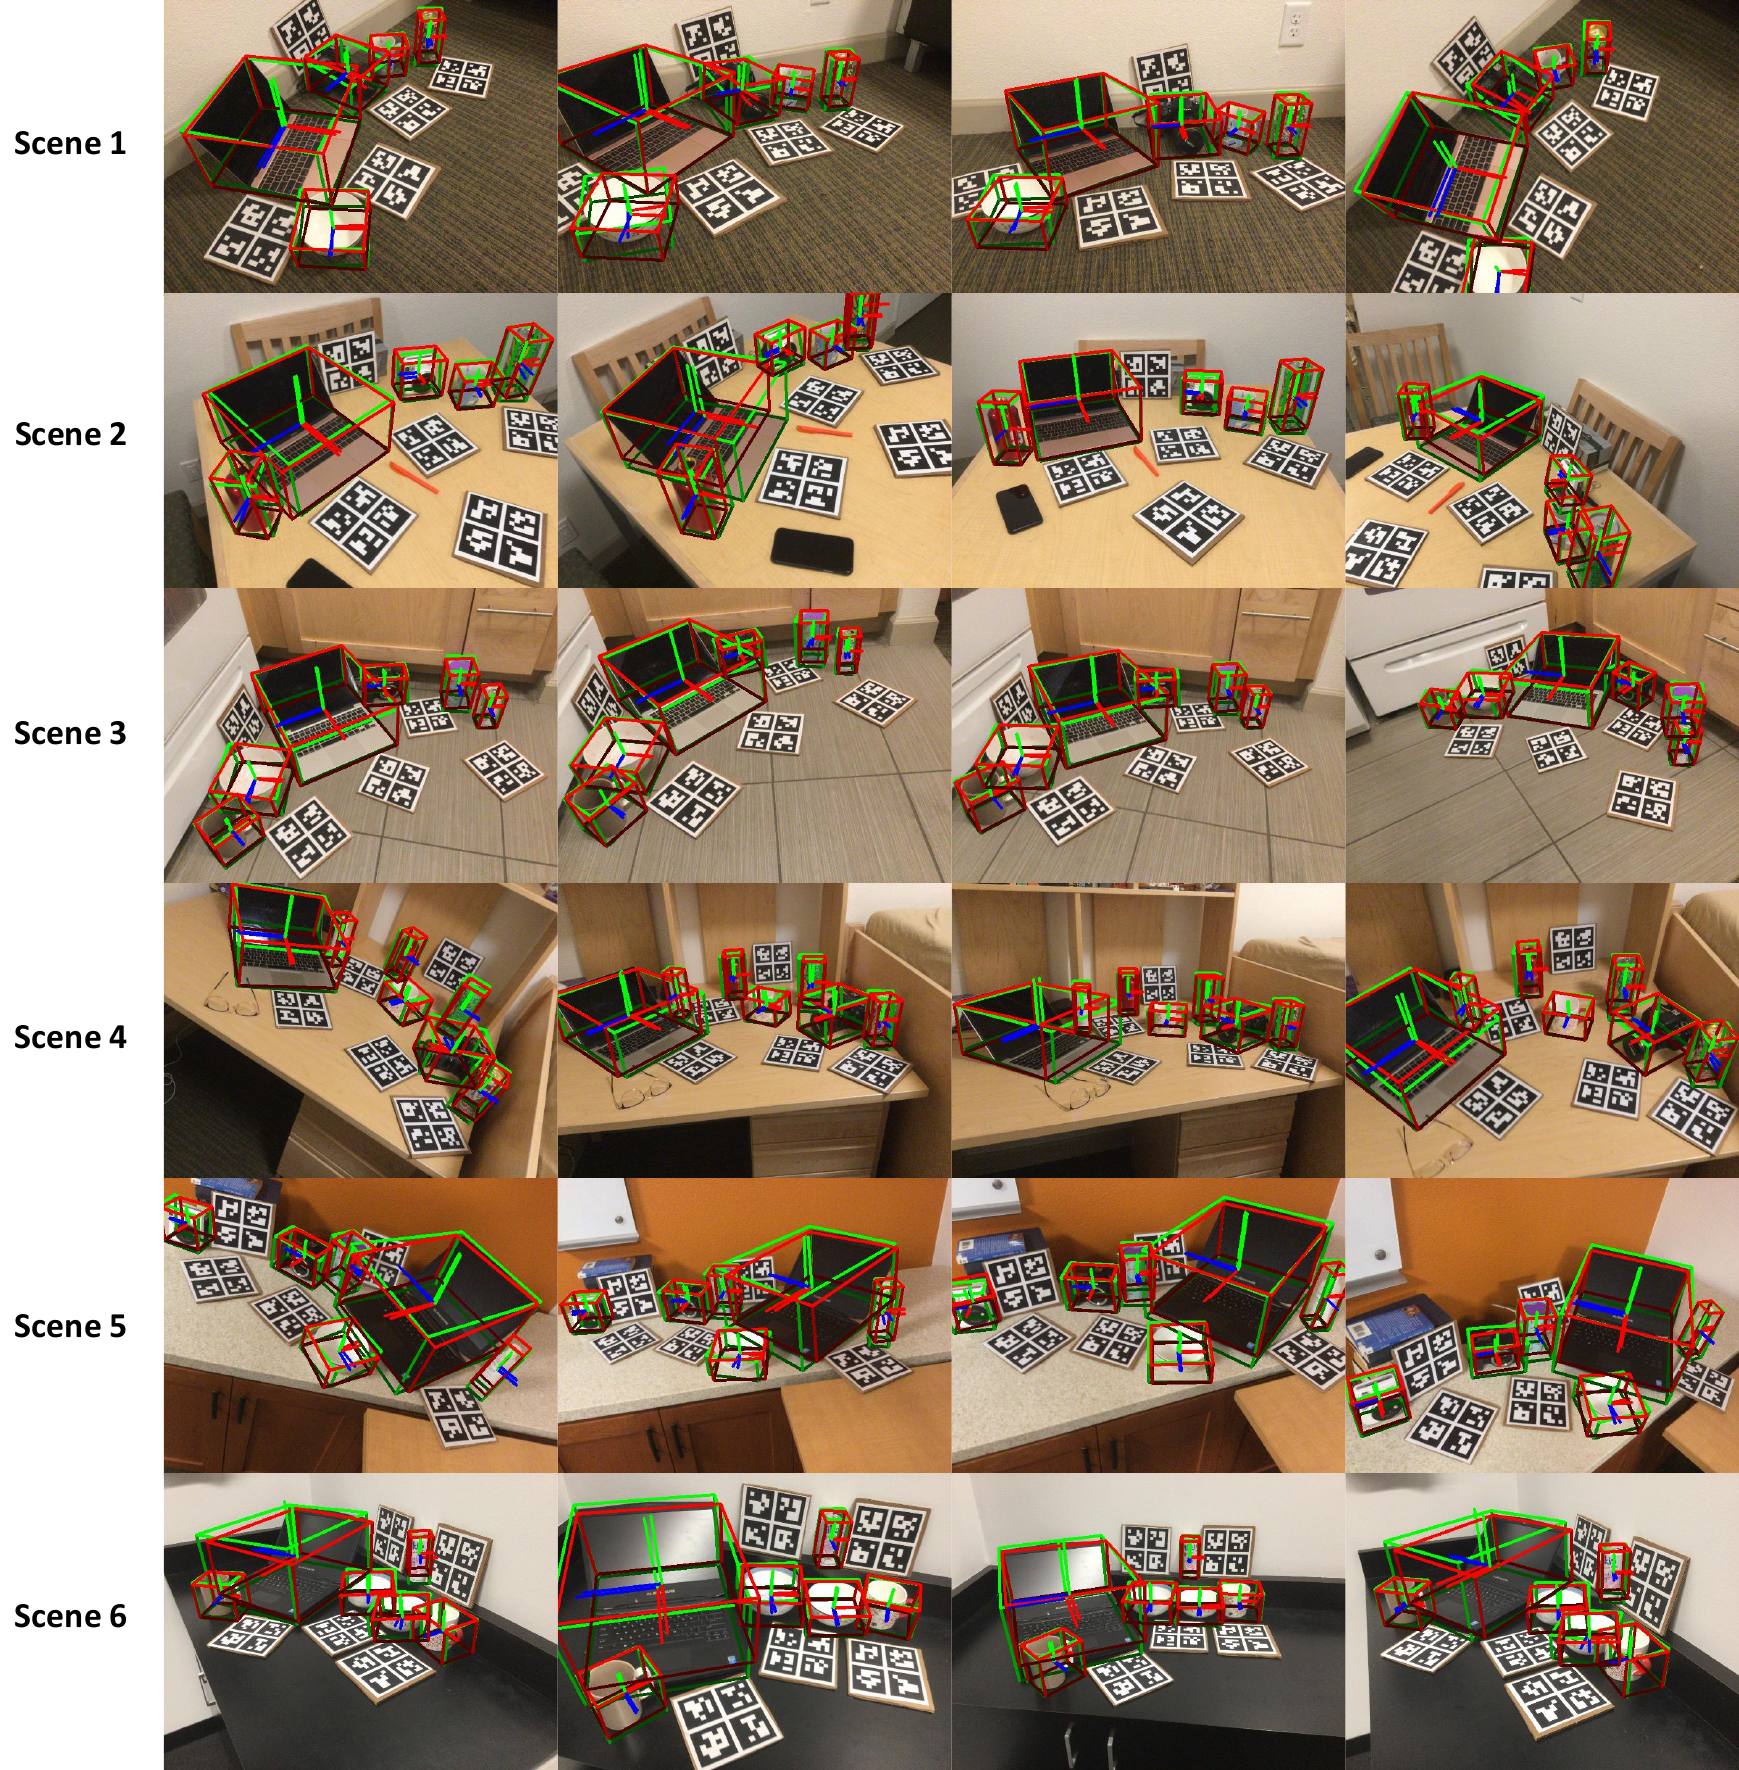}
    \caption{\textbf{More qualitative results of our AG-Pose on the REAL275 dataset.} Red/Green indicates the predicted/gt results.}
    \label{fig:more_viz} 
    \end{center}
    \vspace{-0.25in}
\end{figure*}
