# Supplementary material for: Instance-Adaptive and Geometric-Aware Keypoint Learning for Category-Level 6D Object Pose Estimation
Source: arXiv:2403.19527 source file (2024-03-28)
Supplement: Supplementary file 2 [file ab_supp.tex]

\begin{table}[h]
    \setlength{\tabcolsep}{4pt}
    \caption{\textbf{
        Comparisons between models with different $N_{kpt}$.}
        }
    \label{tab:ab_supp}
    \centering
    \begin{tabular}{c|cc|c|c|c}
        \hline
        $N_{kpt}$ & $IoU_{75}$         & $5^{\circ} \, 2 \, \textbf{cm}$             & Memory & Parameters & Speed(FPS) \\ \hline
        16     & 78            & 47.9          & 11.6G      & 207,529,575        & 30.61      \\
        32     & 78.3          & 48.8          & 12.1G      & 207,541,863        & 30.33      \\
        64     & \textbf{79.7} & 51            & 13.4G      & 207,566,439        & 29.88      \\
        96     & 79.5          & \textbf{54.7} & 14.4G      & 207,591,015        & 27.98      \\
        128    & 78.8          & 52.8          & 16.4G      & 207,615,591        & 27.58      \\ \hline
        \end{tabular}
\end{table}
